# Supplementary material for: Generating Holistic 3D Human Motion from Speech
Source: arXiv:2212.04420 source file (2023-06-17)
Supplement: Supplementary file 1 [file SEC_08_appendix.tex]

% \input{tables/sym.tex}
